# Supplementary material for: First-order kinetics bottleneck during photoinduced ultrafast insulator-metal transition in 3D orbitally-driven Peierls insulator CuIr$_{2}$S$_{4}$
Source: arXiv:2104.03698 source file (2021-04-08)
Supplement: Supplementary file 1 [file CuIr2S4-multipulse-10-supplemental.pdf]

# First-order kinetics bottleneck during photoinduced ultrafast insulator-metal transition in 3D orbitally-driven Peierls insulator $CuIr_2S_4$: Supplemental Material

M. Naseska,[1] P. Sutar,[1] Y. Vaskivskyi,[1] I. Vaskivskyi,[1] D. Vengust,[1]
D. Svetin,[1] V. V. Kabanov,[1] D. Mihailovic,[1,2] and T. Mertelj[1,2,*]

[1] *Complex Matter Department, Jozef Stefan Institute, Jamova 39, 1000 Ljubljana, Slovenia*
[2] *Center of Excellence on Nanoscience and Nanotechnology Nanocenter (CENN Nanocenter), Jamova 39, 1000 Ljubljana, Slovenia*

(Dated: March 2, 2021)

### A. DC photoinduced resistance

The DC resistance was measured by means of a four tip scanning tunneling microscope with optical access as described in Ref. [1]. Four blunt tungsten tips were positioned along a line on a cleaved sample surface[1] in the 4-point configuration with the outer current tips at a $\sim 20$ $\mu$m distance and the inner voltage tips at a $\sim 5$ $\mu$m distance. With the tips in-place the sample was first cooled to $T = 50$ K that was the lowest $T$ at which we could reliably measure 4-point resistance in our setup due to the increasing contact resistance at low $T$. At $T = 50$ K the sample was exposed to femtosecond laser pulse train[2] illumination with an elliptical-Gaussian spatial fluence profile with the size of $85 \times 105$ $\mu$m$^2$ FWHM. After the initial illumination at $F_{\mathrm{peak}} = 50$ $\mu$J/cm$^2$/pulse the resistance first dropped on a ten-seconds timescale due to the combination of photoinduced and laser heating effects. The illuminated spot position was then optimized to obtain the lowest 4-point resistance. The resistance dropped from the initial $\sim 19$ M$\Omega$ and stabilized at $\sim 9.4$ M$\Omega$ under illumination. Upon blocking the laser illumination the resistance increased to $\sim 13$ M$\Omega$ due to the absence of the laser heating and the instant photoconductance. Further exposure at increased $F$ resulted in more abrupt resistance drops, but affected the resulting dark resistance, measured upon laser blocking, only slightly. Assuming that the thickness of the photoinduced disordered conducting phase equals the laser penetration depth of 40 nm (see Section F) we estimate the resistivity drop from the initial estimated bulk value, $\rho_{\mathrm{init}} \sim 10^5$ $\Omega$cm, to $\rho_{\mathrm{DWC}} \sim 10^3$ $\Omega$cm. This is an order of magnitude larger than reported previously for the case of X-rays illumination at $T = 8.5$ K[2] and comparable to the case of high-energy ion illumination at $T = 40$ K.[3]

[1] The crystal orientation of the cleaved surface was not determined.
[2] At 1.55 eV photon energy and 100kHz repetition rate.

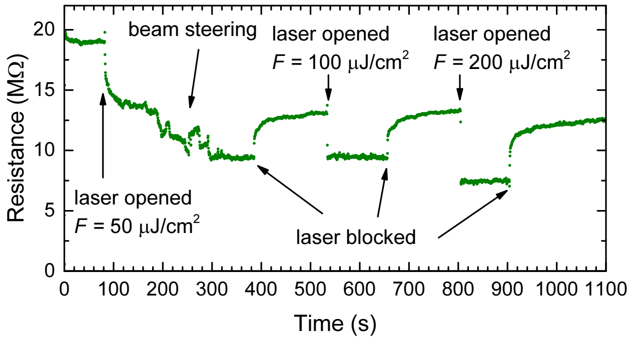


Figure S1. The 4-point DC resistance at $T = 50$ K as a function of the laser illumination.

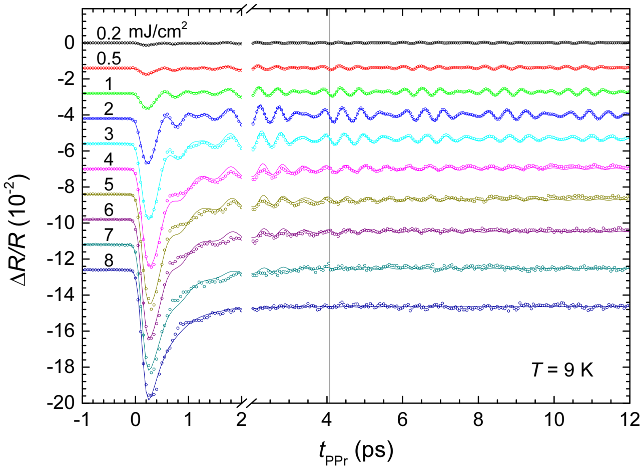


Figure S2. The DECP model fits to the transient reflectivity as a function of $F_{\mathrm{P}}$ in the low-$T$ phase. The traces are vertically offset for clarity and the thin lines correspond to the DECP model fit.

### B. DECP model fits

To analyze the signal we fit the data using the displacive-excitation of coherent-phonons (DECP) model

[4] where the transient reflectivity is given by

$$\frac{\Delta R}{R} = (A_{\mathrm{e}} + \sum A_{\mathrm{O}i}) \int_0^\infty G(t-u) e^{-u/\tau_{\mathrm{e}}} du$$
$$- \sum A_{\mathrm{O}i} \int_0^\infty G(t-u) e^{-\gamma_i u} [\cos(\Omega_i u)$$
$$- \beta_i \sin(\Omega_i u)] du$$
$$+ \sum A_{\mathrm{e}j} \int_0^\infty G(t-u) e^{-u/\tau_j} du, \qquad (1)$$

where $\beta_i = (1/\tau_e - \gamma_i)/\Omega_i$ and $G(t) = \sqrt{2/\pi}\tau_{\mathrm{p}} \exp(-2t^2/\tau_{\mathrm{p}}^2)$ with $\tau_{\mathrm{p}}$ being the effective pump-probe pulse cross-correlation width. For the fits we fixed $\tau_{\mathrm{p}}$ to 150 fs, which is longer than the experimental pump autocorrelation width of $\sim 80$ fs, to take into account the experimentally observed risetime in the MC phase at $T = 245$ K.

In the model the coherent modes are driven by an exponentially relaxing electronic mode with the relaxation time $\tau_{\mathrm{e}}$ and the amplitude, $A_{\mathrm{e}}$. $A_{\mathrm{e}}$ represents the coupling of the electronic mode to the optical reflectivity while the couplings to different oscillatory modes are implicitly included in the parameters $A_{\mathrm{O}i}$. $A_{\mathrm{O}i}$, $\Omega_i$, $\gamma_i$ are the oscillating modes amplitudes, frequencies and damping factors, respectively, while $A_{\mathrm{e}j}$ and $\tau_j$ are the amplitudes and relaxation times of additional exponentially relaxing modes.

The experimental transient reflectivity in the low-$T$ disordered weakly conducting phase can be fairly described (see Figure S2) assuming an exponentially relaxing electronic component with the relaxation time $\tau_{\mathrm{e}}$ in the picosecond range that drives five oscillatory lattice modes. An additional slowly relaxing exponential component with $\tau_1 \sim \infty$ needs to be included to completely describe the relaxation at long delays. [5]

For the three weakest coherent modes (O3, O4, O5) the corresponding dampings showed large scattering and caused fit instability. In order to prevent the adverse influence to the fit convergence we fixed the three weakest modes $\gamma_i$ to 0.03 THz. The fixed values of the dampings were chosen to approximately correspond to the values determined for the strongest modes O1 and O2 in the middle of the relevant $F$ ranges. Since the scan lengths are comparable or shorter than $\gamma_i^{-1}$ this introduces only some systematic bias to the amplitudes of these modes at higher $F$, but does not affect significantly their frequencies and the other-components fit parameters.

Above $F_{\mathrm{P}} \sim 3.5$ mJ/cm$^2$ the DECP model fails to fit the data completely and does not converge unless we fix also the dampings of the the strongest modes.

### C. Fluence dependence at higher $T$

The the transient reflectivity nonlinearities as a function of $F_P$ of the low-$T$ symmetry-broken phase at elevated $T$ appear similar to the low-$T$ behavior but at significantly lower $F_{\mathrm{c}} \sim 1.5 - 2$ mJ/cm$^2$ as shown in Figure S4.

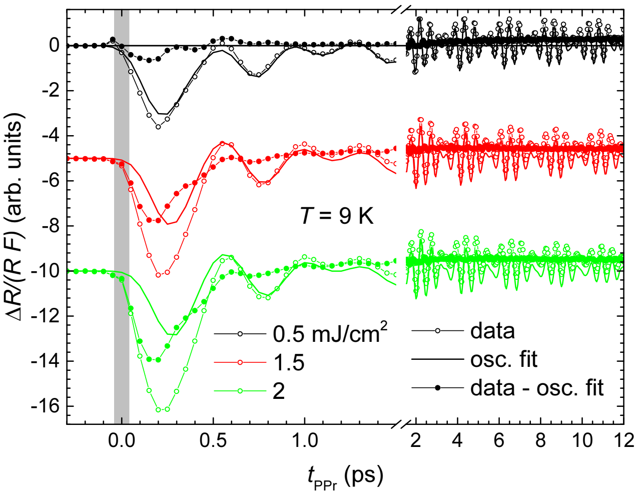


Figure S3. The exponential components near $F_{\mathrm{ce}}$ obtained by subtracting the coherent oscillators fit components from the data. The gray bar represents the pump autocorrelation width of $\sim 80$ fs.

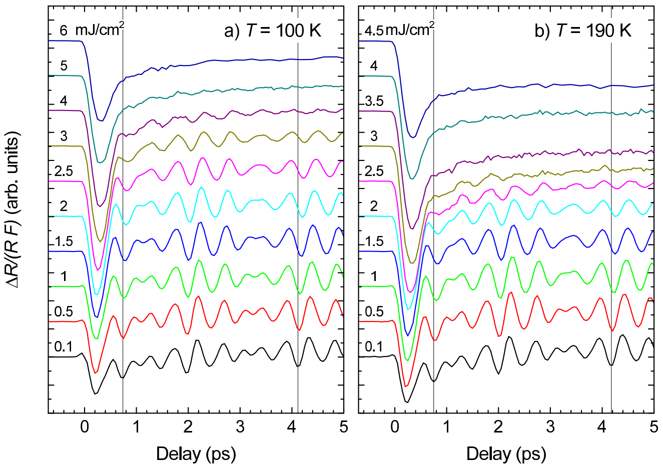


Figure S4. The $F$-normalized transient reflectivity as a function of the P pulse fluence in the low-$T$ IT state at higher temperatures. The behavior is identical to the low-$T$ case, but, with a decreased $F_{\mathrm{c}}$.

The transient reflectivity in the high-$T$ MC phase shows virtually linear scaling with increasing $F$ as shown in Figure S5.

### D. Multi-pulse transient reflectivity

Multipulse transient reflectivity at $F_{\mathrm{D}} = 8.1$ mJ/cm$^2$ is shown in Figure S6. The behavior is similar to that at

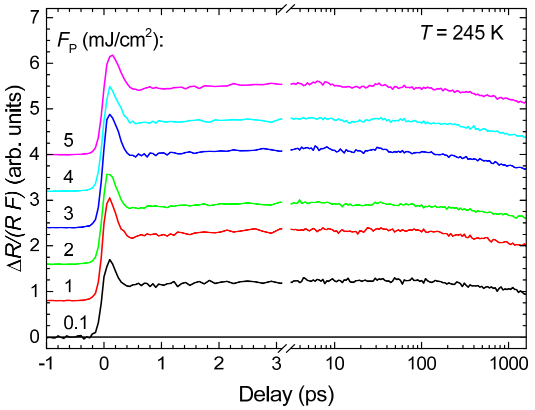


Figure S5. The $F$-normalized transient reflectivity as a function of the P-pulse fluence in the metallic cubic state. The traces are offset vertically for clarity. Note that the invariance of the $F$-normalized traces with $F$ corresponds to the linear scaling with $F$.

slightly lower $F_D = 6.8$ mJ/cm$^2$ presented in the main paper, but the coherent oscillation recovery is somewhat slower.

Comparison of the multipulse transient reflectivity with the standard two-pulse one measured at identical $F_P$ is shown in Figure S7. A simulation assuming the maximal possible $T$ gradient cannot reproduce the strong experimental dephasing.

The suppression of the coherent phonon oscillations is delayed for $t_{DPr} \sim 0.6$ ps with respect to the D-pulse arrival and does not depend on the $t_{DP}$ delay as shown in Figure S8. However, the negative/positive transient reflectivity swings are suppressed/enhanced already on a $\sim$ 0.2-ps $t_{DPr}$ timescale. This is attributed to a weak D-pulse impulsive excitation of the coherent phonons.

### E. Multi-pulse transient reflectivity fits

In order to fit the data within the model (1) an additional slow exponential component with finite but long, $\tau_2 \gg t_{PPr}$ was employed.

The effective temperatures, $T_{O1}$ and $T_{O2}$, were obtained from the frequencies of the coherent phonons O1 and O2, respectively using anharmonic [5] extrapolation of the low-$T$ equilibrium softening above $T_{IM}$. At $F_D = 6.8$ mJ/cm$^2$ (see Fig. 6 (d) in the main text) they stay below $\sim$ 500 K dropping to $\sim T_{IM}$ after $\sim$ 200 ps (see also Figure S9). At $t_{DP} = 5$ $\mu$s delay, just before the arrival of the next pulse sequence, the effective temperatures remain below $T \sim 100$ K in the full $F_D$ range (see Figure S9).

| | I-phase gap (eV) | $\Delta V/V$ (%)[a] |
|---|---|---|
| $VO_2$ | 0.6 [9] | 0.1 [10] |
| $V_2O_3$ | 0.2-0.75 [11] | -1.29 [12] |
| $CuIr_2S_4$ | 0.15 [7] | 0.7 [13] |

[a] Across the IM transition.

Table I. Comparison of selected structural and electronic parameters in $VO_2$, $V_2O_3$ and $CuIr_2S_4$

### F. Transient heating estimate

We estimate the equivalent fluence, $F_{c-th}$, to reach the high-$T$ MC phase thermally using the static optical [6, 7] and $T$-dependent heat capacity [8] data. Taking the optical penetration depth, $\alpha_{sc}^{-1} \sim 40$ nm, from single crystal data, [7] and $R = 0.4$, one obtains[3] $F_{c-th} = 2.1$ mJ/cm$^2$, which is $\sim$ 30 % smaller than the experimental $F_c \sim 3$ mJ/cm$^2$. Taking the polycrystaline sample optical penetration depth, $\alpha_{pc}^{-1} \sim 80$ nm and reflectivity $R = 0.17$, [6] one obtains $F_{c-th} = 3.2$ mJ/cm$^2$, which is closer to the experimental $F_c \sim 3$ mJ/cm$^2$.

The room-$T$ reflectivity of our sample mirror-like cleaved surface of $R = 0.19$ at $\hbar\omega = 1.55$ eV is significantly smaller than the published [7] single crystal reflectivity and closer to the the polished polycrystaline samples [8] reflectivity. Since the preparation of the single crystal surface [7] was not specified and our Raman data [5] indicate that as-grown or polished surfaces show poor quality the single crystal $\alpha_{sc}^{-1}$ obtained from Ref. [7] might not be reliable.

Assuming that $T_{IM}$ is reached at $F_c$ we estimate the maximal transient temperature in the multi-pulse experiments to be $T \sim 400$ K at $F_D \sim 6.8$ mJ/cm$^2$. The effective phonon temperatures, $T_{O1}$ and $T_{O2}$ (see Figure 6 (d) in the main text), appear consistent with the estimate.

### G. Calculation of excitation densities

Using the same optical data as above we estimate the absorbed photon number densities and obtain $n_{phot}/F \sim 2-3 \times 10^{20}$ cm$^{-1}$mJ$^{-1}$. Assuming creation of only one[4] electron-hole pair per photon we obtain the photoexcited carriers plasma frequency of $\sim$ 0.4 eV at $F_{ce} = 0.6$ mJ/cm$^2$. This is larger than the insulating gap (see Table I). It is therefore conceivable, that the localized Ir $d$-band carriers are delocalized due to the Mott transition and the gap is washed out.

---

[3] Including the transition enthalpy [8] of 3.5 kJ/mol.
[4] With 1.55 eV photon energy up to $\sim$ 10 pairs are possible.

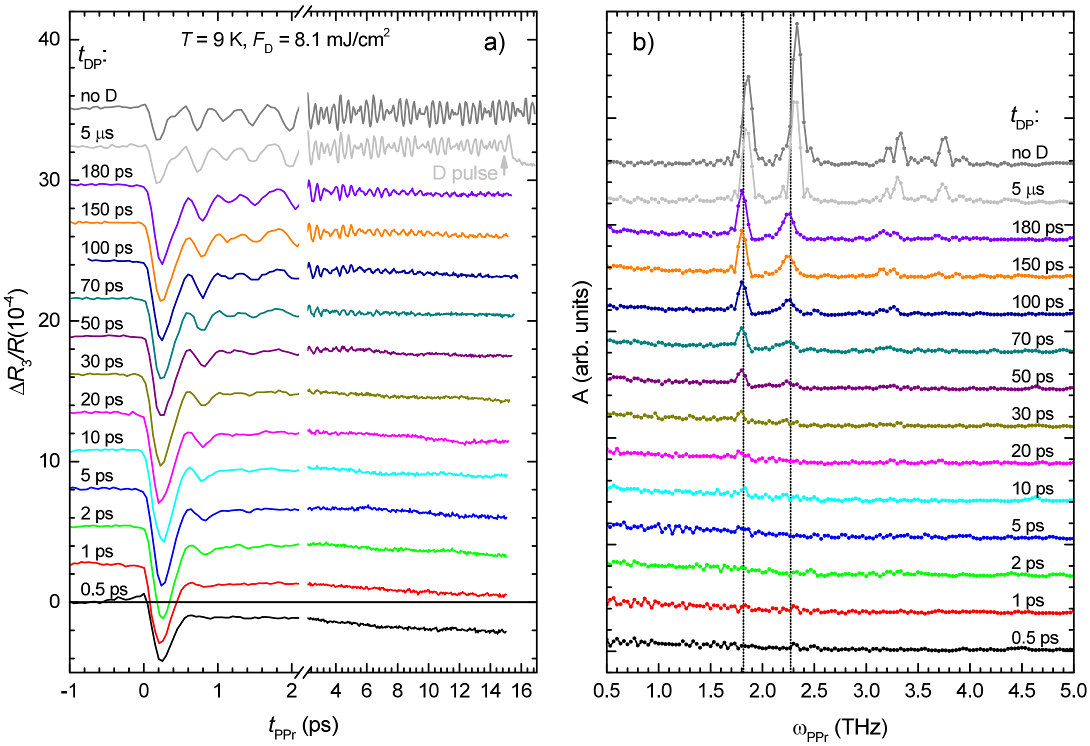


Figure S6. Multi-pulse transient reflectivity as a function of the delay between the D and P pulses, $t_{\mathrm{DP}}$, from sample S2 at $F_{\mathrm{D}} = 8.1\ \mathrm{mJ/cm^2}$. The arrow at $t_{\mathrm{DP}} = 5\ \mu\mathrm{s}$ indicates arrival of the subsequent D pulse. The traces are vertically offset for clarity.

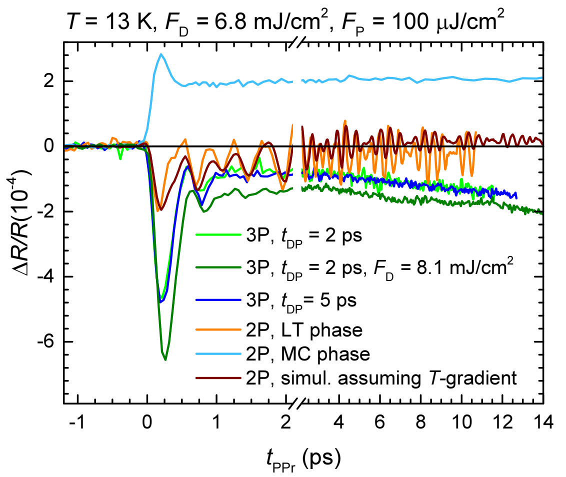


Figure S7. Comparison of the selected multipulse transients to the equilibrium two-pulse transients in both phases. A simulated transient assuming the maximum possible $T$-gradient (13 K - $T_{\mathrm{IM}}$) within the probed volume is shown for comparison. The trace is calculated by averaging $T$-dependent equilibrium transient traces across the full low-$T$ phase $T$-range.

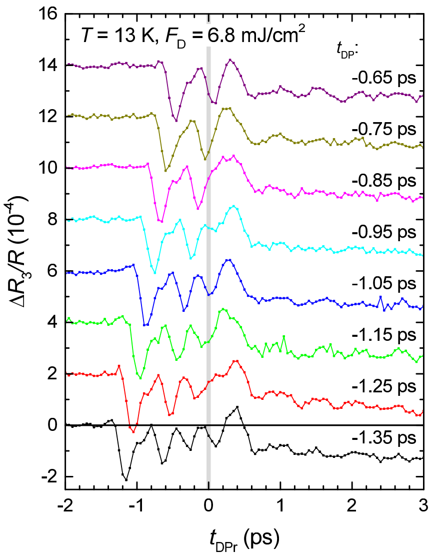


Figure S8. Multi-pulse transient reflectivity as a function of delay between the D and P pulses, $t_{\mathrm{DP}}$, in sample S2. The vertical gray bar corresponds to the arrival and the length of the D pulse.

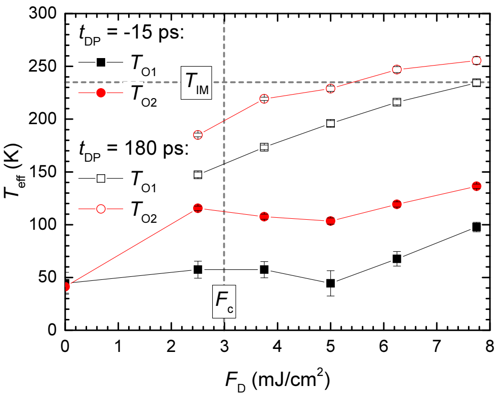


Figure S9. The effective temperatures of the two strongest modes as a function of the D-pulse fluence 15 ps before (equivalent to $\sim 5\ \mu$s after) and 180 ps after the D pulse arrival.

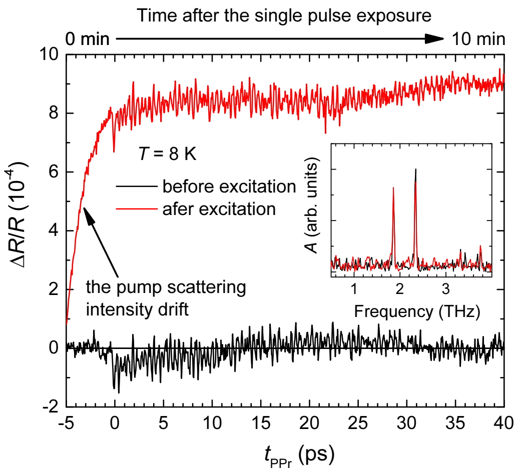


Figure S10. Low-$F$ transient reflectivity before and immediately after a strong single-pulse excitation in sample S1. The delay-independent background due to the pump scattering leaking into the detector was determined before excitation and subtracted from both scans by means of the lock-in offset function. The top axis indicates the acquisition times of data points at the particular delays. The Fourier-transform amplitude of the scans is shown in the inset.

## H. Single shot experiments

To search for existence of any long-lived metastable infrared-light induced state a set of single-strong-pulse experiments was also performed in sample S1. In these experiments the excitation volume was first exposed (at $T = 8$ K) to a single 50-fs optical pulse (at 1.55-eV photon energy) with $F \sim 5$ mJ/cm$^2$. After that a sequence of low-$F$ scans was acquired. These scans revealed a time scale of minutes during which we observed a strong change of the pump scattering intensity[5]. This hindered acquisition of the transient reflectivity scans due to unstable background (see Figure S10), however, the coherent-phonons spectra obtained from such scans show no detectable changes as shown in the inset to Figure S10.

It is unclear whether the slow pump scattering intensity variation can be related to a slow low-$T$ weakly conducting phase [14] relaxation observed also in the DC transport experiment (see Figure S1) since the thermal dilatation of microscopic cracks at the sample surface can also cause a similar effect.

## References

* tomaz.mertelj@ijs.si

[1] Y. A. Gerasimenko, I. Vaskivskyi, M. Litskevich, J. Ravnik, J. Vodeb, M. Diego, V. Kabanov, and D. Mihailovic, Nature materials **18**, 1078 (2019).
[2] T. Furubayashi, H. Suzuki, T. Matsumoto, and S. Nagata, Solid state communications **126**, 617 (2003).
[3] M. Koshimizu, H. Tsukahara, and K. Asai, Nuclear Instruments and Methods in Physics Research Section B: Beam Interactions with Materials and Atoms **267**, 1125 (2009).
[4] H. Zeiger, J. Vidal, T. Cheng, E. Ippen, G. Dresselhaus, and M. Dresselhaus, Physical Review B **45**, 768 (1992).
[5] M. Naseska, P. Sutar, D. Vengust, S. Tsuchiya, M. Čeh, D. Mihailovic, and T. Mertelj, Physical Review B **101**, 165134 (2020).
[6] M. Hayashi, M. Nakayama, T. Nanba, T. Matsumoto, J. Tang, and S. Nagata, Physica B: Condensed Matter **281**, 631 (2000).
[7] N. Wang, G. Cao, P. Zheng, G. Li, Z. Fang, T. Xiang, H. Kitazawa, and T. Matsumoto, Physical Review B **69**, 153104 (2004).
[8] T. Hagino, T. Tojo, T. Atake, and S. Nagata, Philosophical Magazine B **71**, 881 (1995).
[9] T. C. Koethe, Z. Hu, M. W. Haverkort, C. Schüßler-Langeheine, F. Venturini, N. B. Brookes, O. Tjernberg, W. Reichelt, H. H. Hsieh, H.-J. Lin, C. T. Chen, and L. H. Tjeng, Phys. Rev. Lett. **97**, 116402 (2006).
[10] M. Marezio, P. Dernier, D. McWhan, and J. Remeika, Materials Research Bulletin **5**, 1015 (1970).
[11] V. Simic-Milosevic, N. Nilius, H.-P. Rust, and H.-J. Freund, Phys. Rev. B **77**, 125112 (2008).
[12] P. Rozier, A. Ratuszna, and J. Galy, Zeitschrift für anorganische und allgemeine Chemie **628**, 1236 (2002).
[13] T. Furubayashi, T. Matsumoto, T. Hagino, and S. Nagata, Journal of the Physical Society of Japan **63**, 3333 (1994).
[14] W. Sun, T. Kimoto, T. Furubayashi, T. Matsumoto,

[5] The background signal from the detector due to the pump beam with the probe beam blocked.

S. Ikeda, and S. Nagata, Journal of the Physical Society of Japan **70**, 2817 (2001).
